# Supplementary material for: A Relation Algebra for Term Rewriting: A differential approach to sequential reduction (Revised Version)
Source: arXiv:2312.02996 source file (2023-11-30)
Supplement: Supplementary file 1 [file appendix.tex]

% Carattere dimensione 12
\documentclass[12pt]{report}

\input{../macros}

\begin{document}
\appendix \,

\end{document}
